# Supplementary material for: Task Agnostic and Post-hoc Unseen Distribution Detection
Source: arXiv:2207.13083 source file (2022-07-26)
Supplement: Supplementary file 1 [file 07_algorithms.tex]

% \newcommand{\UMOS}{\ensuremath{\mbox{\sc UMOS}}}
% \begin{algorithm}
% \caption{Unsupervised MOS algorithm}\label{UMOS}
% \begin{algorithmic}[1]
% \State $f$ := feature extractor
% \State $g$ := logistic regression detector
% \State $\mathcal{C}$ := the number of clustering
% \State 
% \Procedure{UMOS$_{train}$}{$ f, g, \mathcal{X}, \mathcal{C}$}
%   \State $\mathcal{Z} \gets f(\mathcal{X})$ \Comment{feacture extraction}
%   \State estimator = GaussianMixture($\mathcal{C}$) \Comment{with full covariance matrix}
%   \State estimator.train($\mathcal{Z}$)
%   \State Clusters = estimator.predict($\mathcal{Z}$)

%   \State C$_{train}$, C$_{valid}$, C$_{test}$ = split-data-from-clusters($\mathcal{Z}$, Clusters)
%   \State train($g$, C$_{train}$, C$_{valid}$, C$_{test}$) \Comment{ trained by group-wise-softmax-loss }

%   \State \textbf{return} $g$
% \EndProcedure
% \State 
% \Procedure{UMOS$_{test}$}{$f, g, \mathcal{X}_{in}, \mathcal{X}_{out}$}
%     \State $\mathcal{Z}_{in}$, $\mathcal{Z}_{out}$ = $f$($\mathcal{X}_{in}$), $f$($\mathcal{X}_{out}$)
%     \State logit$_{in}$, logit$_{out}$ = $g$($\mathcal{Z}_{in}$), $g$($\mathcal{Z}_{out}$)
%     \State mos\_score$_{in}$ = calculate-mos-score(logit$_{in}$) \Comment{Calculated by equation (1)}
%     \State mos\_score$_{out}$ = calculate-mos-score(logit$_{out}$)

%   \State \textbf{return} mos\_score$_{in}$, mos\_score$_{out}$ 
% \EndProcedure

% \end{algorithmic}
% \end{algorithm}

\begin{algorithm}
\caption{Unsupervised Mahalanobis algorithm}\label{Umahalanobis}
\begin{algorithmic}[1]
\State $f$ := penultimate layer
\State $\mathcal{C}$ := the number of clustering
\State 
\Procedure{U-Mahalanobis$_{train}$}{$ f, \mathcal{X}, \mathcal{C}$}
   \State $\mathcal{Z} \gets f(\mathcal{X})$ \Comment{feacture extraction}
   \State estimator $\gets$ GaussianMixture($\mathcal{C}$) \Comment{with full covariance matrix}
   \State estimator.train($\mathcal{Z}$)
   \State clusters $\gets$ estimator.predict($\mathcal{Z}$)
   \State $\mu$, ${\Sigma}$ $\gets$ estimator.means, estimator.precisions \Comment{same with equation (4)}

   \State \textbf{return} $\mu$, ${\Sigma}$
\EndProcedure
\State 
\Procedure{U-Mahalanobis$_{test}$}{$f$, $\mathcal{X}_{in}, \mathcal{X}_{out}, \mu, {\Sigma}$}
    \State $\mathcal{Z}_{in}$, $\mathcal{Z}_{out}$ $\gets$ $f$($\mathcal{X}_{in}$), $f$($\mathcal{X}_{out}$)

    \State $conf_{in}$ $\gets$ get-mahalanobis-score($f, \mathcal{X}_{in}, \mu, {\Sigma}$) \Comment{calculated by equation (5)}
    \State $conf_{out}$ $\gets$ get-mahalanobis-score($f, \mathcal{X}_{out}, \mu, {\Sigma}$)
    
   \State \textbf{return} $conf_{in}$, $conf_{out}$
\EndProcedure
\State

\end{algorithmic}
\end{algorithm}

 \begin{algorithm}
\caption{TAUOOD algorithm}\label{tauood}
\begin{algorithmic}[1]
\State $M$ := number of clusters
\State $conf_{in}$, $conf_{out}$ := mahalanobis score from $algorithm \,\, 1$ for different values of $M$
\State $mode$ := type of ensembling
\State
\Procedure{TAUOOD}{$conf_{in}$, $conf_{out}$, $mode$, $M$}
   \State Initialize
   \If{$mode$ $is$ seesaw}
   \State $totalscore$ $\gets$ $concatenation( conf_{in}[n], conf_{out}[n])$
   \State $k$ $\gets$ get number of clusters in $totalscore$
   \State $\mu_{seasaw}$ $\gets$ $ {1 \over \mathcal{C}} \sum_{n=1}^{\mathcal{C}} totalscore $
   \State $control$ $\gets$ get number of clusters upper $\mu_{seasaw}$ in $totalscore$
   \If{$control$ $\geq$ $\frac{k}{2}$ }
   \State $\hat{\mathcal{X}}_{in}$, $\hat{\mathcal{X}}_{out}$ $\gets$ take highest $M$ clusters in $totalscore$
   \Else
   \State $\hat{\mathcal{X}}_{in}$, $\hat{\mathcal{X}}_{out}$ $\gets$ take lowest $M$ clusters in $totalscore$
   \EndIf
   
   \ElsIf{$mode$ $is$ trimmed average}
   \State $\hat{\mathcal{X}}_{in}$, $\hat{\mathcal{X}}_{out}$ $\gets$ drop least and maximum score in $conf_{in}$, $conf_{out}$
   \ElsIf{$mode$ $is$ top}
   \State $\hat{\mathcal{X}}_{in}$, $\hat{\mathcal{X}}_{out}$ $\gets$ get highest $M$ mahalanobis scores in $conf_{in}$, $conf_{out}$
   \ElsIf{$mode$ $is$ bottom}
      \State $\hat{\mathcal{X}}_{in}$, $\hat{\mathcal{X}}_{out}$ $\gets$ get lowest $M$ mahalanobis scores in $conf_{in}$, $conf_{out}$
   \Else \Comment{averaging of confidence scores}
   \State $\hat{\mathcal{X}}_{in}$, $\hat{\mathcal{X}}_{out}$ $\gets$ $conf_{in}$, $conf_{out}$

   \EndIf

   \State {$ \hat{\mu}_{in} \gets {1 \over \mathcal{C}} \sum_{n=1}^{\mathcal{C}} \hat{\mathcal{X}}_{in}[n] $}
   \State {$ \hat{\mu}_{out} \gets {1 \over \mathcal{C}} \sum_{n=1}^{\mathcal{C}} \hat{\mathcal{X}}_{out}[out] $}

   \State {$ \hat{\Sigma}_{in} \gets {1 \over \mathcal{C}} \sum_{n=1}^{\mathcal{C}} (\hat{\mathcal{X}}_{in}[n] - \hat{\mu}_{in})(\hat{\mathcal{X}}_{in}[n] - \hat{\mu}_{in})^{\top}  $}
   \State {$ \hat{\Sigma}_{out} \gets {1 \over \mathcal{C}} \sum_{n=1}^{\mathcal{C}} (\hat{\mathcal{X}}_{out}[n] - \hat{\mu}_{out})(\hat{\mathcal{X}}_{out}[n] - \hat{\mu}_{out})^{\top}  $}

   \State \textbf{return} $\hat{\mu}_{in}, \hat{\mu}_{out}, \hat{\Sigma}_{in}, \hat{\Sigma}_{out}$
\EndProcedure
\State

\end{algorithmic}
\end{algorithm}
