# Supplementary material for: Task Agnostic and Post-hoc Unseen Distribution Detection
Source: arXiv:2207.13083 source file (2022-07-26)
Supplement: Supplementary file 3 [file tap_mos.tex]

% \newcommand{\UMOS}{\ensuremath{\mbox{\sc UMOS}}}
% \begin{algorithm}
% \caption{Unsupervised MOS algorithm}\label{UMOS}
% \begin{algorithmic}[1]
% \State $f$ := feature extractor
% \State $g$ := logistic regression detector
% \State $\mathcal{C}$ := the number of clustering
% \State 
% \Procedure{UMOS$_{train}$}{$ f, g, \mathcal{X}, \mathcal{C}$}
%   \State $\mathcal{Z} \gets f(\mathcal{X})$ \Comment{feacture extraction}
%   \State estimator = GaussianMixture($\mathcal{C}$) \Comment{with full covariance matrix}
%   \State estimator.train($\mathcal{Z}$)
%   \State Clusters = estimator.predict($\mathcal{Z}$)

%   \State C$_{train}$, C$_{valid}$, C$_{test}$ = split-data-from-clusters($\mathcal{Z}$, Clusters)
%   \State train($g$, C$_{train}$, C$_{valid}$, C$_{test}$) \Comment{ trained by group-wise-softmax-loss }

%   \State \textbf{return} $g$
% \EndProcedure
% \State 
% \Procedure{UMOS$_{test}$}{$f, g, \mathcal{X}_{in}, \mathcal{X}_{out}$}
%     \State $\mathcal{Z}_{in}$, $\mathcal{Z}_{out}$ = $f$($\mathcal{X}_{in}$), $f$($\mathcal{X}_{out}$)
%     \State logit$_{in}$, logit$_{out}$ = $g$($\mathcal{Z}_{in}$), $g$($\mathcal{Z}_{out}$)
%     \State mos\_score$_{in}$ = calculate-mos-score(logit$_{in}$) \Comment{Calculated by equation (1)}
%     \State mos\_score$_{out}$ = calculate-mos-score(logit$_{out}$)

%   \State \textbf{return} mos\_score$_{in}$, mos\_score$_{out}$ 
% \EndProcedure

% \end{algorithmic}
% \end{algorithm}
